# Supplementary material for: Evaluating Trustworthiness of Online News Publishers via Article Classification
Source: arXiv:2401.01781 source file (2024-01-03)
Supplement: Supplementary file 1 [file appendix.tex]

% \section{Domain List}
%\begin{appendices}

For the reader's convenience, Table~\ref{tab:domains} reports the news outlets' domains we used to create our dataset. The labels on topic and source trustworthiness cannot be made public because they are NewsGuard's proprietary data, which the authors of the work have a license to. We would be happy to work out an agreement with NewsGuard to release the tags partially. 

We will be happy to release the trustworthiness classification model in the final version of the paper if accepted.

\begin{table}[t!]
    \centering
    \caption{\label{tab:domains}List of news domains considered in the final dataset}
    \begin{tabular}{ll}
        \textbf{Domain names} \\ \hline
        12up.com & aclu.org \\
        americanprogress.org & bizpacreview.com \\
        californiahealthline.org & cbssports.com \\
        celebritiesdeaths.com & clutchpoints.com \\
        nih.gov & news-front.info \\
        ewg.org & famadillo.com \\
        filthylucre.com & flagandcross.com \\
        harmonyhustle.com & historyfact.in \\
        labourlist.org & nationalrighttolifenews.org \\
        now8news.com & nowtheendbegins.com \\
        on3.com & outsideonline.com \\
        politichome.com & powerofpositivity.com \\
        psypost.org & pulsetoday.co.uk \\
        realrawnews.com & sbnation.com \\
        scoopearth.com & skepticalraptor.com \\
        sportscasting.com & theamericanmirror.com \\
        thecovidblog.com & thegrayzone.com \\
        thelibertytimes.com & thepatriotjournal.com \\
        theplayerstribune.com & theringer.com \\
        thetentacle.com & tnewsnetwork.com \\
        trendingpoliticsnews.com & truthdig.com \\
        unz.com & wavefunction.info \\
        consciousreminder.com & countylocalnews.com \\
        deadspin.com & dreddymd.com \\
        drjockers.com & \\ \hline
    \end{tabular}
\end{table}

% \section{Detailed classification performances}

\begin{figure}[!t]
    \includegraphics[width=0.9\textwidth]{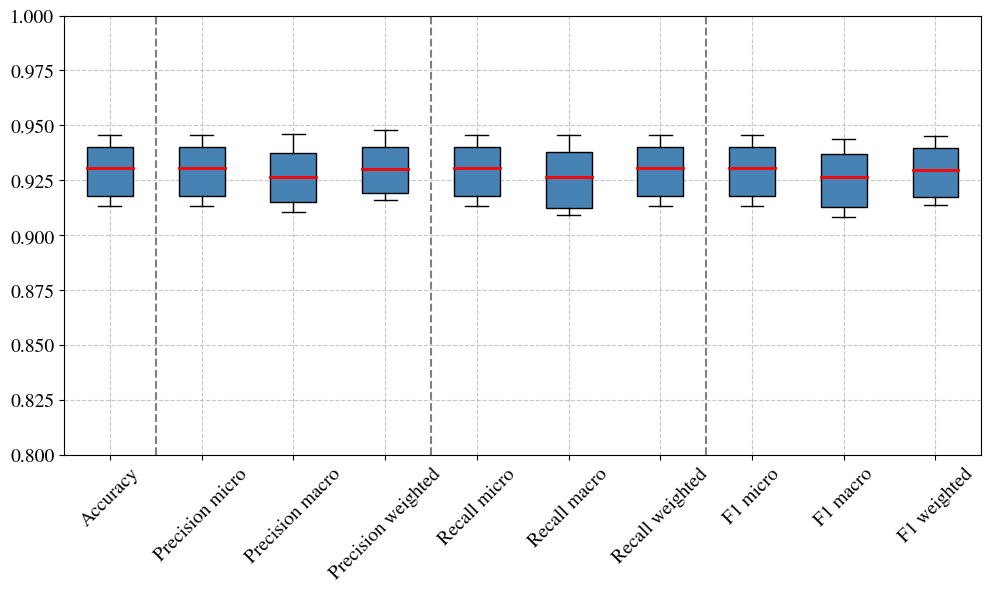}
    \caption{Complete evaluation results Topic Classification\label{fig:topicScores}}
\end{figure}

\begin{figure}[!h]
    \centering
    \includegraphics[width=0.9\textwidth]{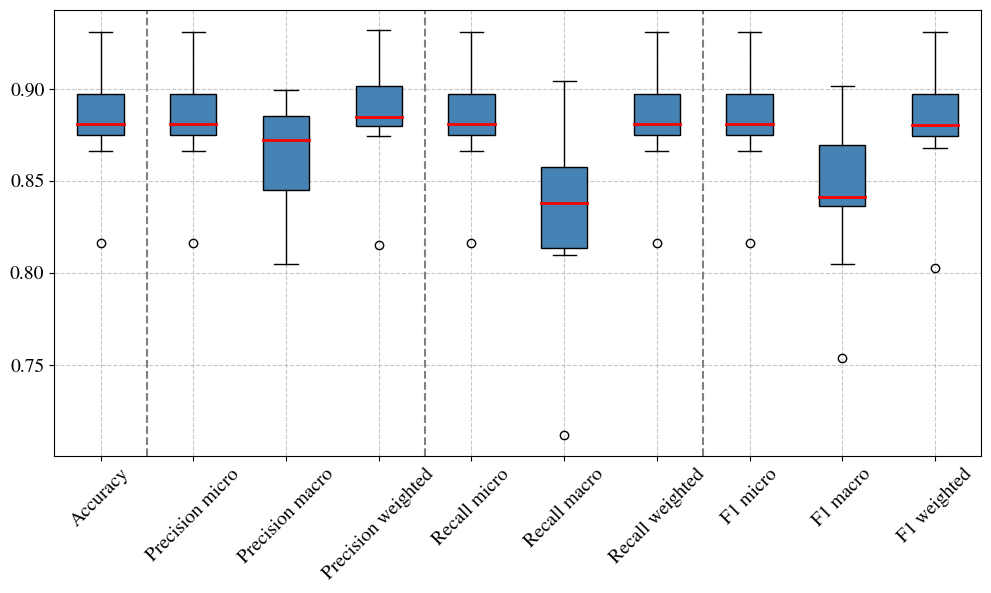}
    \caption{Complete evaluation results for Trustworthiness Classification\label{fig:trustScores}}
\end{figure}

Figure~\ref{fig:topicScores} and Figure~\ref{fig:trustScores} show the performances obtained for the Topic Classification Task and the Trustworthiness Classification Task regarding Accuracy, Precision, Recall and F1.
